# Supplementary material for: Nonlinear association structures in flexible Bayesian additive joint models
Source: arXiv:1708.06337 ancillary file (2017-10-23)
Supplement: Supplementary file 1 [file Supporting_Information.pdf]

# Supplementary Information

Nonlinear association structures in flexible Bayesian additive joint models

Meike Köhler, Nikolaus Umlauf, Sonja Greven

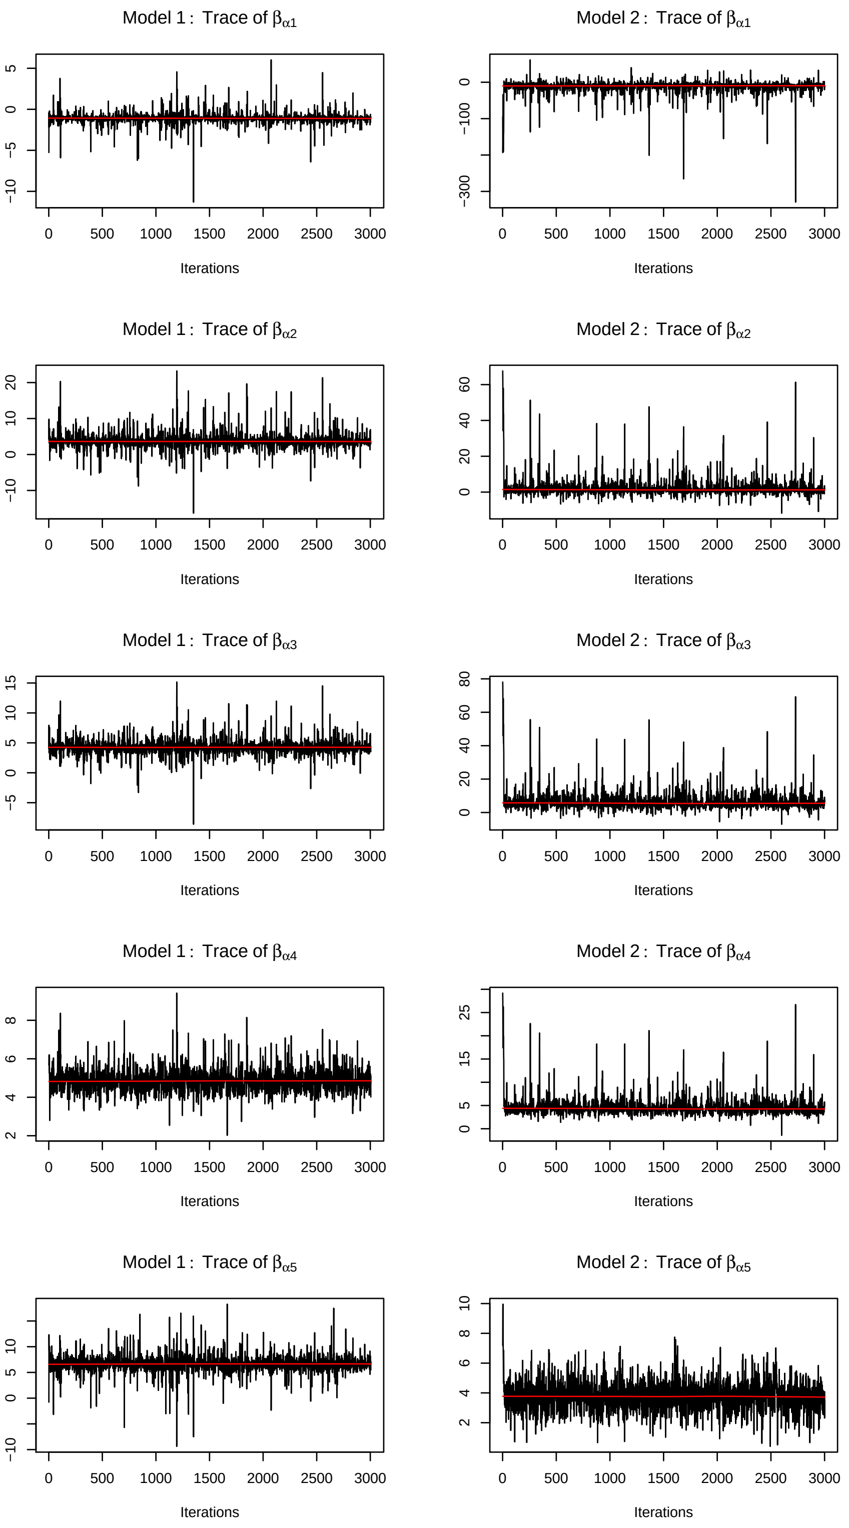


SupplementaryFigure S1: Traceplots of the posterior samples for $\boldsymbol{\beta}_\alpha$ in $\eta_\alpha(\eta_\mu(t))$ from model 1 (left) and model 2 (right).

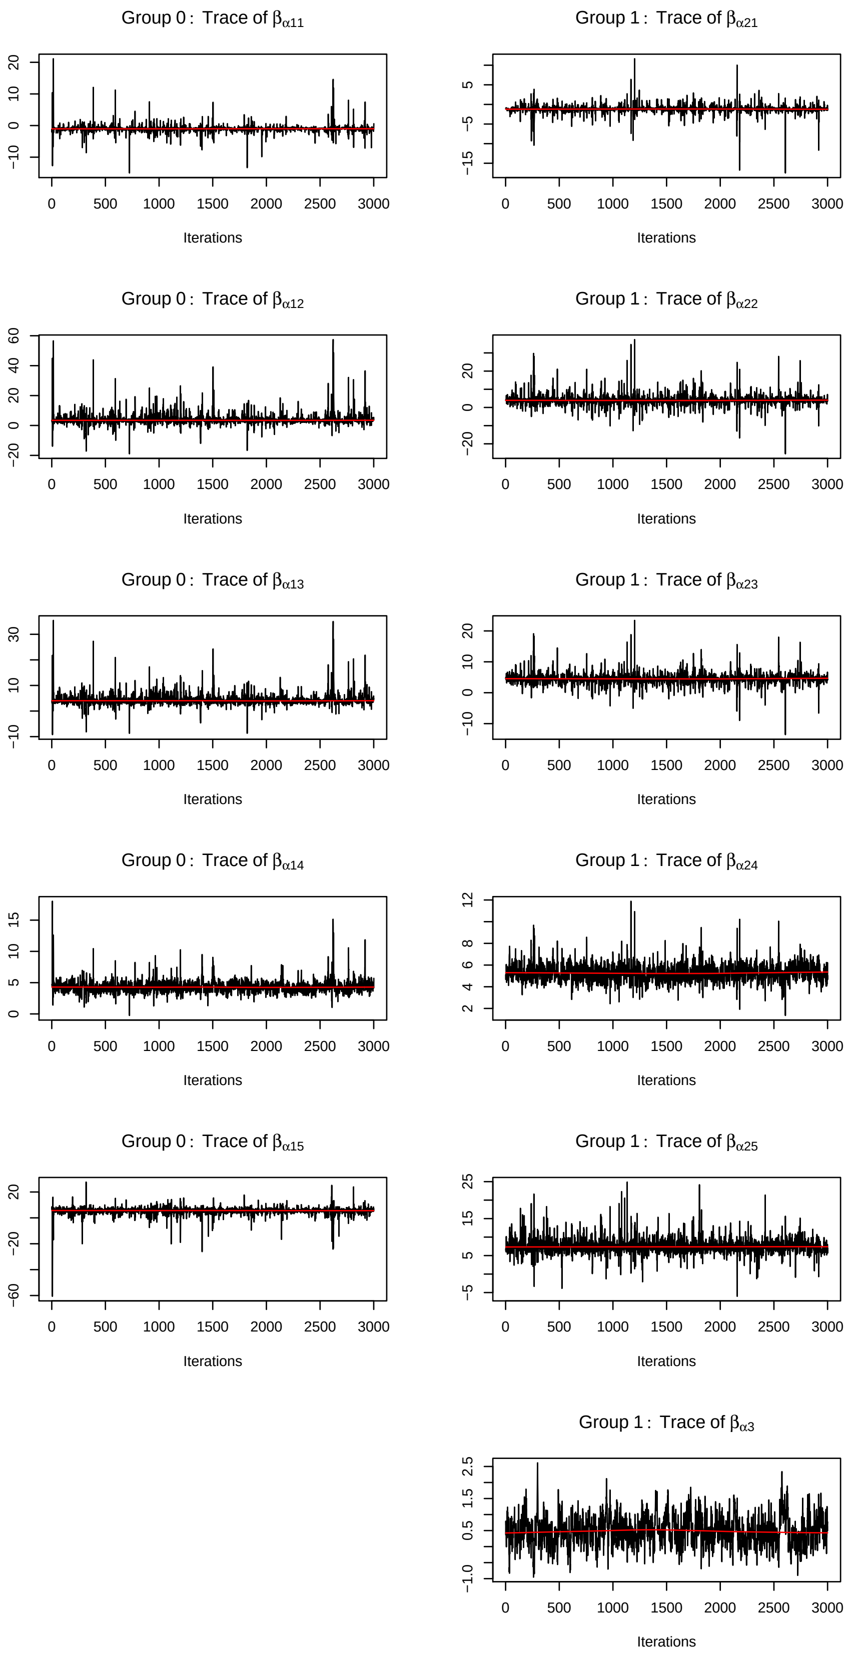


SupplementaryFigure S2: Traceplots of the posterior samples of model 3 for $\boldsymbol{\beta}_\alpha$ in $\eta_\alpha(\eta_\mu(t), g)$ from subjects without an enlarged liver at baseline (left) and with this condition (right). For the latter also a group-specific intercept $\beta_{\alpha 3}$ is estimated.

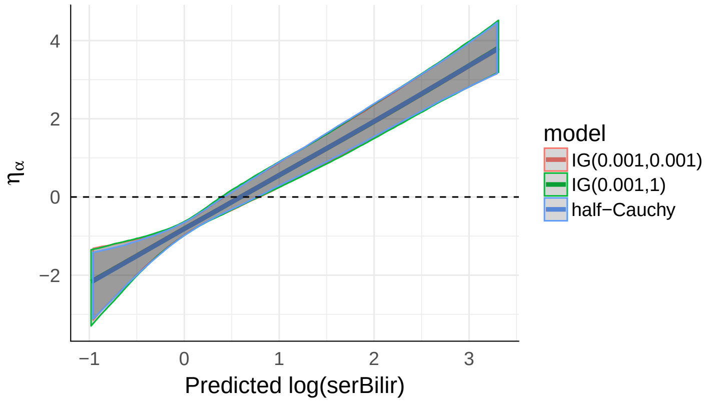


(a)

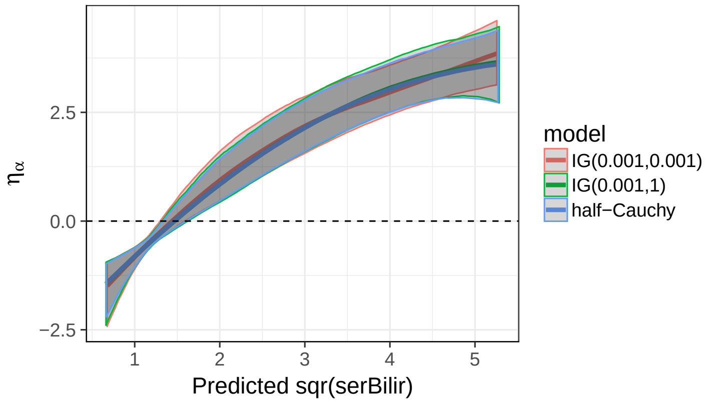


(b)

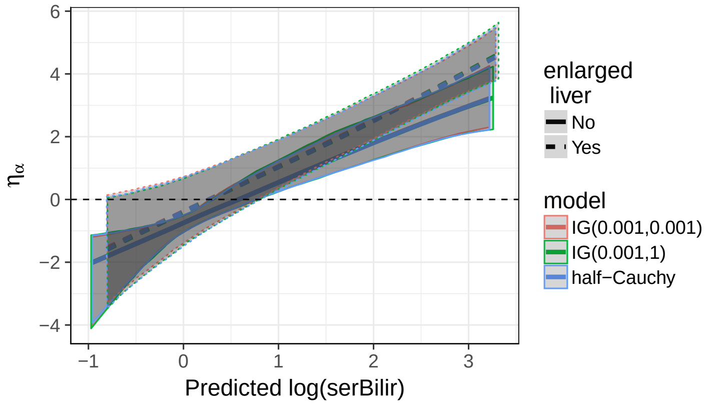


(c)

SupplementaryFigure S3: Results from the sensitivity analysis for the PBC data. Estimated posterior mean of the association $\eta_\alpha(\eta_\mu(t))$ of (a) model 1 (nonlinear estimation of $\log(Bilirubin)$), (b)model 2 (nonlinear estimation of $\sqrt(Bilirubin))$ and (c) model 3 (nonlinear estimation of $\log(Bilirubin)$ of patients with and without enlarged liver at baseline) using as prior distribution for the variance parameters (i) $IG(0.001, 0.001)$, (ii) $IG(0.001, 1)$, and (iii) a half-Cauchy distribution for the variance parameters.
